# Supplementary material for: Improved Sample Complexity Analysis For First Order Bilevel Reinforcement Learning
Source: arXiv:2611.01500 source file (2026-11-01)
Supplement: Supplementary file 2 [file preserved_mechanism_details.tex]

\subsection{Finite-problem validation}

\paragraph{Exact scalar problems.}
The unit-test bandit is closed-form and entropy regularized. The principal
scalar environment is a continuing branching finite MDP with exact
matrix-resolvent occupancy, exact lower and upper derivatives, and exact base
and perturbed responses. Computation uses NumPy float64. Table~\ref{tab:finite-hp}
lists the principal deterministic and stochastic settings.

\begin{table}[ht]
\centering
\caption{Scalar finite-MDP validation settings.}
\label{tab:finite-hp}
\begin{tabularx}{\linewidth}{@{}Xrr@{}}
\toprule
Hyperparameter & Deterministic & Stochastic \\
\midrule
Iterations & 600 & 800 \\
Secant perturbation $c$ & 0.1 & 0.1 \\
Lower step size & 0.2 & 0.15 \\
Upper step size & 0.05 & 0.03 \\
Fragment horizon & population & 128 \\
Lower samples / iteration & population & 256 \\
Outer fragments / iteration & population & 256 total \\
Training replicates & 1 & 5 common seeds \\
Upper domain / prox radius & --- & $[-1,1]$ / 5 \\
\bottomrule
\end{tabularx}
\end{table}

The deterministic bias sweep uses
$c\in\{0.2,0.1,0.05,0.02,0.01,0.005\}$. The variance sweep uses the first five
of these values, 150 repetitions, horizon 16, and 256 total fragments per
repetition. Stochastic horizon calibration tests
$H\in\{16,32,64,128\}$ and selects $H=128$ from exact truncation bias rather
than observed optimization performance.

\paragraph{Fixed-chart neural finite MDP.}
This problem has nine states, three decision contexts, and two actions. Each
context is encoded by two raw features. A fixed affine layer with three tanh
units produces a full-rank $3\times3$ hidden-feature matrix. The action-0
energy is $h(s)^\top\theta$ with trainable $\theta\in\mathbb{R}^3$; the
action-1 energy is fixed to zero, removing additive-logit and hidden-unit
non-identifiability. The chart condition number is 1.238. The experiment uses
float64 autodiff, exact matrix-resolvent occupancy, $\gamma=0.9$, entropy
regularization $\tau=0.5$, and upper regularization 0.3.

The five-seed neural recursion runs 1000 iterations with $c=0.1$, lower and
upper step sizes 0.15 and 0.03, $H=128$, 256 lower samples, 256 total outer
fragments, upper box $[-1,1]^3$, and KL-prox radius 5. Sensitivity sweeps vary
$c$, horizon, batch size, and iteration count while changing one factor at a
time.

\subsection{Controlled Walker Stand campaign}

The frozen Phase-13 campaign uses normalized DeepMind Control Walker Stand,
two parallel environments, common training seeds $0$--$4$, and a requested
25,000 combined interactions per run (25,480 actual). Full chain and no chain
share the complete collection, preference, PPO, and evaluation pipeline; only
the applied value-gap coefficient changes from 1 to 0.

\begin{table}[ht]
\centering
\caption{Frozen Walker Stand policy and PPO settings.}
\label{tab:walker-ppo}
\begin{tabularx}{\linewidth}{@{}XlXl@{}}
\toprule
Setting & Value & Setting & Value \\
\midrule
Policy/value MLPs & separate $2\times1024$ & Activation & tanh \\
Policy distribution & diagonal Gaussian + gSDE & Learning rate & $3\times10^{-4}$ \\
Rollout & $2$ envs $\times1024$ steps & Minibatch & 256 \\
Epochs / rollout & 5 & GAE $\lambda$ & 0.92 \\
Policy/value clip & 0.2 / 0.2 & Value coefficient & 0.5 \\
Entropy coefficient & 0 & Gradient cap & 0.3 \\
Target KL & 0.01 & gSDE frequency & 4 \\
Initial burn-in & 5000 interactions & Evaluation & every 5000, 20 episodes \\
\bottomrule
\end{tabularx}
\end{table}

The reward model is an ensemble of three MLPs. Each consumes concatenated
state and action, has three 256-unit LeakyReLU hidden layers, and a scalar tanh
output. Adam learning rate is $3\times10^{-4}$; preference minibatch size is
128; segment length is 50; reward updates per query block are 50. The frozen
campaign uses current lower-rollout preferences with capacity 128.

The response perturbation is $c=0.09$. Each pair uses a 25\% held-out outer
split and four-step fragments. The actor response update uses a common
empirical Fisher with four Rademacher probes, coefficient 0.1, damping 0.001,
actor learning rate 0.01, and gradient cap 0.3. KL primal--dual control uses
initial coefficient 1, dual learning rate 10, up to ten backtracking steps,
and factor 0.5. The critic uses learning rate $3\times10^{-4}$, two extra
epochs, and gradient cap 10. Diagnostic gates are KL $\le0.01$, scaled
separation $\le10$, pair residual $\le1000$, and zero saturation/instability.
